# Supplementary material for: Optimal Workplace Occupancy Strategies during the COVID-19 Pandemic
Source: arXiv:2204.01444 source file (2022-04-04)
Supplement: Supplementary file 1 [file Appendix.tex]

\section*{Appendix: Estimation of probability of transmission}

In our scheduling optimal presence rate problem, the parameter $\beta$ denotes the probability or risk of infection of any susceptible individual per contact with exactly one infected individual. In a more simpler way, how likely an arbitrary employee to be infected in his/her workplace if there is one infected co-worker.  

Realistic estimation of this parameter is very important. Because it would create large uncertainty in the outcomes of the optimization problem.

Though from its theoretical definition, it might look simpler, but in practice defining the risk of infection is very complicated. The risk of infections depends on several individual-based factors like: \\
$(i)$ type of interaction, 
$(ii)$ the duration of interaction, 
$(iii)$ the degree of personal protection maintained during interactions, etc.

However, if the time series data of number of infected employees is available, then it is possible to estimate this parameter using a mechanistic model. Unfortunately, we do not have such data. Therefore we have to rely on the estimates of this parameter from previous study. 

It is also to be noted that these factors also depend on the type of organizations we are interested in. Apart from this, there are several pathogen dependent factors like 
$(i)$ the routes of transmission of the disease,
$(ii)$ infective dose (D50), etc. which play a significant role in determining the realistic estimate of the probability of infection.

Based on available evidences, SARS-COV-2 can be transmitted in three ways:

\textbf{1. Contact transmission:}
Virus can be transmitted when someone comes into direct contact of an infected individual or touches a contaminated surface. During initial phases of the pandemic, it was thought that this route of transmission might play a significant contribution in transmitting the disease. However, latest experimental study \cite{medicine2020covid,mondelli2021low} suggests that contribution of this route of transmission is almost negligible except in health-care setting.

\textbf{2. Droplet transmission:}
During talking, singing, yelling, etc. the viral particles are emitted. The average length of the diameter of  droplet is greater than 5 m. Due to the larger size of droplet, they fall to ground within 2m from the source. For this reason, WHO, CDC recommended to maintain social distancing to reduce the transmission risk.

\textbf{3. Aerosol transmission:}   
The particle of size less than 5  m are characterized as aerosol. Aerosol can suspend in the air over longer distance and longer time than droplet. Researchers have also measured particle sizes of infectious aerosols and have shown that pathogens are most commonly found in small particle aerosol, which are airborne and breathable \cite{medicine2020covid}. Initially transmission through aerosol did not get much attention. However, growing evidences \cite{morawska2020time} suggest that in indoor settings aerosol transmission is the main route for disease transmission.   

Based on the available findings discussed above regarding the routes of disease transmission, it is clear that if we concentrate on the settings like offices, private organizations, schools where people maintain social distancing and wear mask during the office hour, then transmission through aerosol is found out to be the major route of disease transmission.

Recently, a research group from Max Plank Institute for Chemistry, Germany quantified the infection risk of COVID-19 through aerosol transmission in indoor environments \cite{lelieveld2020model}. They estimated the infection risk for different indoor environments like office, classroom, choir practice, reception, etc. based on available data of human aerosol emission, SARS-CoV-2 viral loads, infective dose and other parameters related to structure of the indoor environments, and degree of personal protection etc.     

In this study, four types of indoor environments: (i) Office, (ii) Classroom, (iii) Choir practice, and (iv) Reception are considered. For each of these indoor environment, they considered four scenarios and calculated the risk of infection in the presence of only one infected individual. 

However, we concentrate only on the Office setting. For office setting, it is assumed that the room size is 40 square meter, Room height is 3 m, number of susceptible present in the room is 4, and exposure duration is 16 hrs.

%In the following table we present the parameters and their ranges that are used in [4] to compute the infection risk. There ranges of parameters are taken from previously available estimates. 
%
%Parameters
%Value
%Range
%Unit
%Diameter of aerosol
%5 
%2- 10
%m
%Virus lifetime in aerosol
%1.7
%0.6-2.6
%Hours
%Concentration from breathing/speaking 
%0.1/1.1
%(0.06-1)/ (0.06-6)
%cm-3
%Respiratory rate 
%10
%5-20
%L/min
%Viral load “highly infectious”
%5 x 108
%108-109
%RNA Copies/cm3
%Viral load “super infectious”
%5x109
%109-1010
%RNA Copies/cm3
%Infective dose (D50)
%316
%100-1000
%RNA copies
%Room Area 
%40
%-
%m2
%Room Height
%3
%-
%m
%Susceptible persons in room 
%4
%-
%persons
%Passive ventilation rate 
%0.35
%0-1
%Hour-1
%Active ventilation rate 
%2
%2-9
%Hour-1
%Face mask filter efficiency 
%-
%0-0.95
%
%Time of exposure
%16
%
%Hours

Based on ventilation rate and mask efficiency, five scenarios are considered:

1. Standard (Passive ventilation): Rate of ventilation is 0.35 per hour, without mask efficiency.

2. Active ventilation:  Rate of ventilation is 2 per hour, without mask efficiency.

3. Active ventilation with medium efficient mask: Rate of ventilation is 2 per hour, with 70% mask efficiency.

4. Active ventilation with high efficient mask: Rate of ventilation is 2 per hour, with 95% mask efficiency.

5. High volume air filtration only: High-Efficiency Particulate Air (HEPA) filters with the rate 9 per hour.

Based on the above parameter ranges, in the following table we present the risk of infection in presence of highly infectious index subject (i.e the infectious person with viral load $5\times 10^8$) and super infectious index subject  (i.e the infectious person with viral load $5\times 10^9$) for five different scenarios.

\begin{table}[h!]
	\tabcolsep 7pt
	\centering
	\begin{tabular}{p{3cm} p{1cm} p{1cm} p{1cm} p{1cm} p{1cm}}
		\hline\hline
		 & \textbf{S1} & \textbf{S2} & \textbf{S3}  & \textbf{S4} & \textbf{S5}\\
		[0.5ex]
		\hline
		\textbf{Highly infectious} & \small{19} & \small{7.3} & \small{2.3} & \small{0.4} & \small{2} \\\\
		\textbf{Super infectious} & \small{88} & \small{53} & \small{20} & \small{3.7} & \small{19} \\\\
		%p & Fraction of kit & 1(single model) & []\\\\
		\hline
	\end{tabular}
	\caption{ Risk of infection ($\%$) for five different scenarios}
	\label{table:risk_of_infection}
\end{table}

Scenario 1 is very unlikely, because it represents that the room with closed windows (i.e with air volume exchange rate 0.35 per hour) and nobody is wearing mask. Scenario 2 can be considered in such a situation where mask is not mandatory in the office, however during pandemic lifting wearing mask in the office in not expected. The type of organization we are modelling, we can assume that the Scenario 3 and Scenario 4 are the most common scenarios if no other extra information are provided by the organizations (i.e whether they use HEPA in their office or not).  Also we can discard the possibility of super infection, as it not relatively rare than the highly infectious case.

Therefore we can assume the risk of infection in the office between $0.4 \%$ to $2.3\%$. We should keep that in mind that in reality the risk of infection is highly heterogeneous. However, this estimate gives us an average estimate of risk of infection.

%
%References:
%[1] Medicine, The Lancet Respiratory, COVID-19 transmission—up in the air, The Lancet. Respiratory Medicine, 8 (2020): 1159.
%
%[2] Mondelli, M. U., Colaneri, M., Seminari, E. M., Baldanti, F. and Bruno, R., Low risk of SARS-CoV-2 transmission by fomites in real-life conditions, The Lancet Infectious Diseases, 21 (2021): e112.
%
%[3] Morawska, L. and Milton, D. K., It is time to address airborne transmission of coronavirus disease 2019 (COVID-19), Clinical Infectious Diseases, 71 (2020): 2311-2313.
%
%[4] Lelieveld, J.,  Helleis, F., Borrmann, S., Cheng, Y., Drewnick, F., and Haug, G., Klimach, T.,  Sciare, J., Su, H., and Poschl, U., Model calculations of aerosol transmission and infection risk of COVID-19 in indoor environments, International journal of environmental research and public health, 17 (2020): 8114.
